# Supplementary material for: The Power of Input: Benchmarking Zero-Shot Sim-To-Real Transfer of Reinforcement Learning Control Policies for Quadrotor Control
Source: arXiv:2410.07686 source file (2024-12-26)
Supplement: Supplementary file 1 [file appendix.tex]

\appendix

\section{Technical Details}
\clearpage

\subsection{Observation Space Analysis}

\begin{figure}[h]
    \centering
    \includegraphics[width=\textwidth]{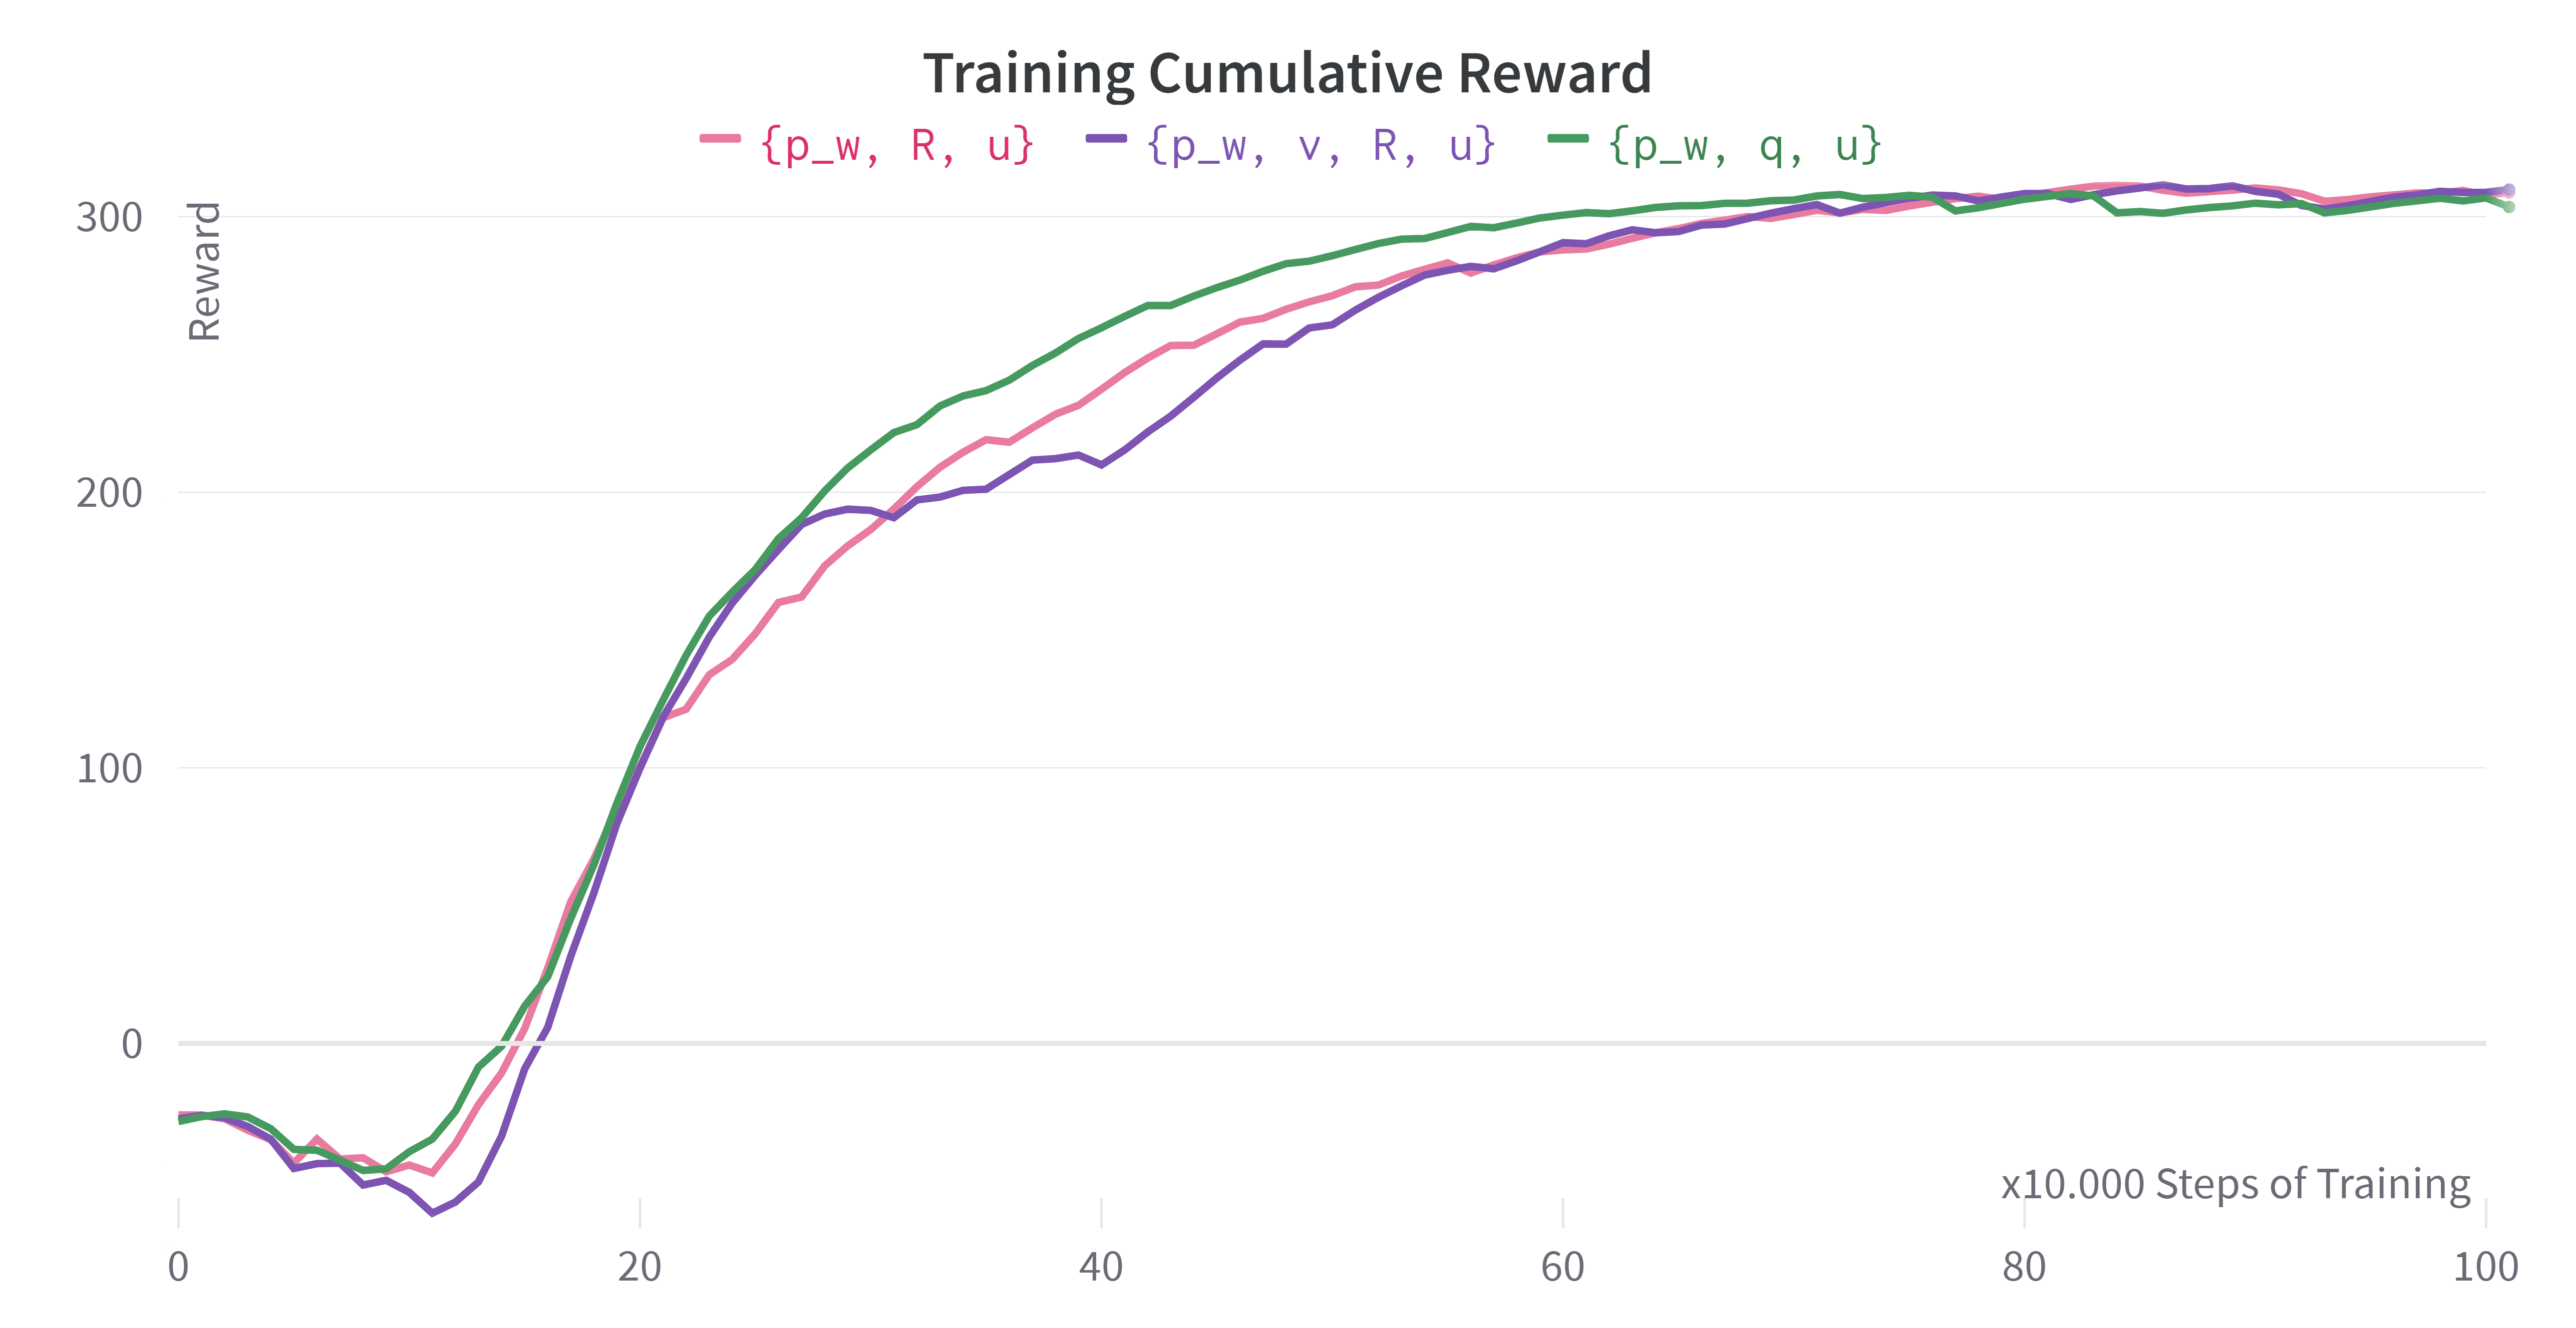}
    \caption{Learning curves of the ablation study models. This plot reports the training cumulative reward of $\{ \mathbf{e}_\mathbf{w}, \mathbf{R},  \mathbf{u}\}$, $\{ \mathbf{e}_\mathbf{w}, \mathbf{v_w}, \mathbf{R},  \mathbf{u}\}$ and $\{ \mathbf{e}_\mathbf{w}, \mathbf{q},  \mathbf{u}\}$.}
    \label{fig:enter-label}
\end{figure}

\input{tables/abl_v_q}

\clearpage

\subsection{Window Length Analysis}

\begin{figure}[h]
    \centering
    \includegraphics[width=\textwidth]{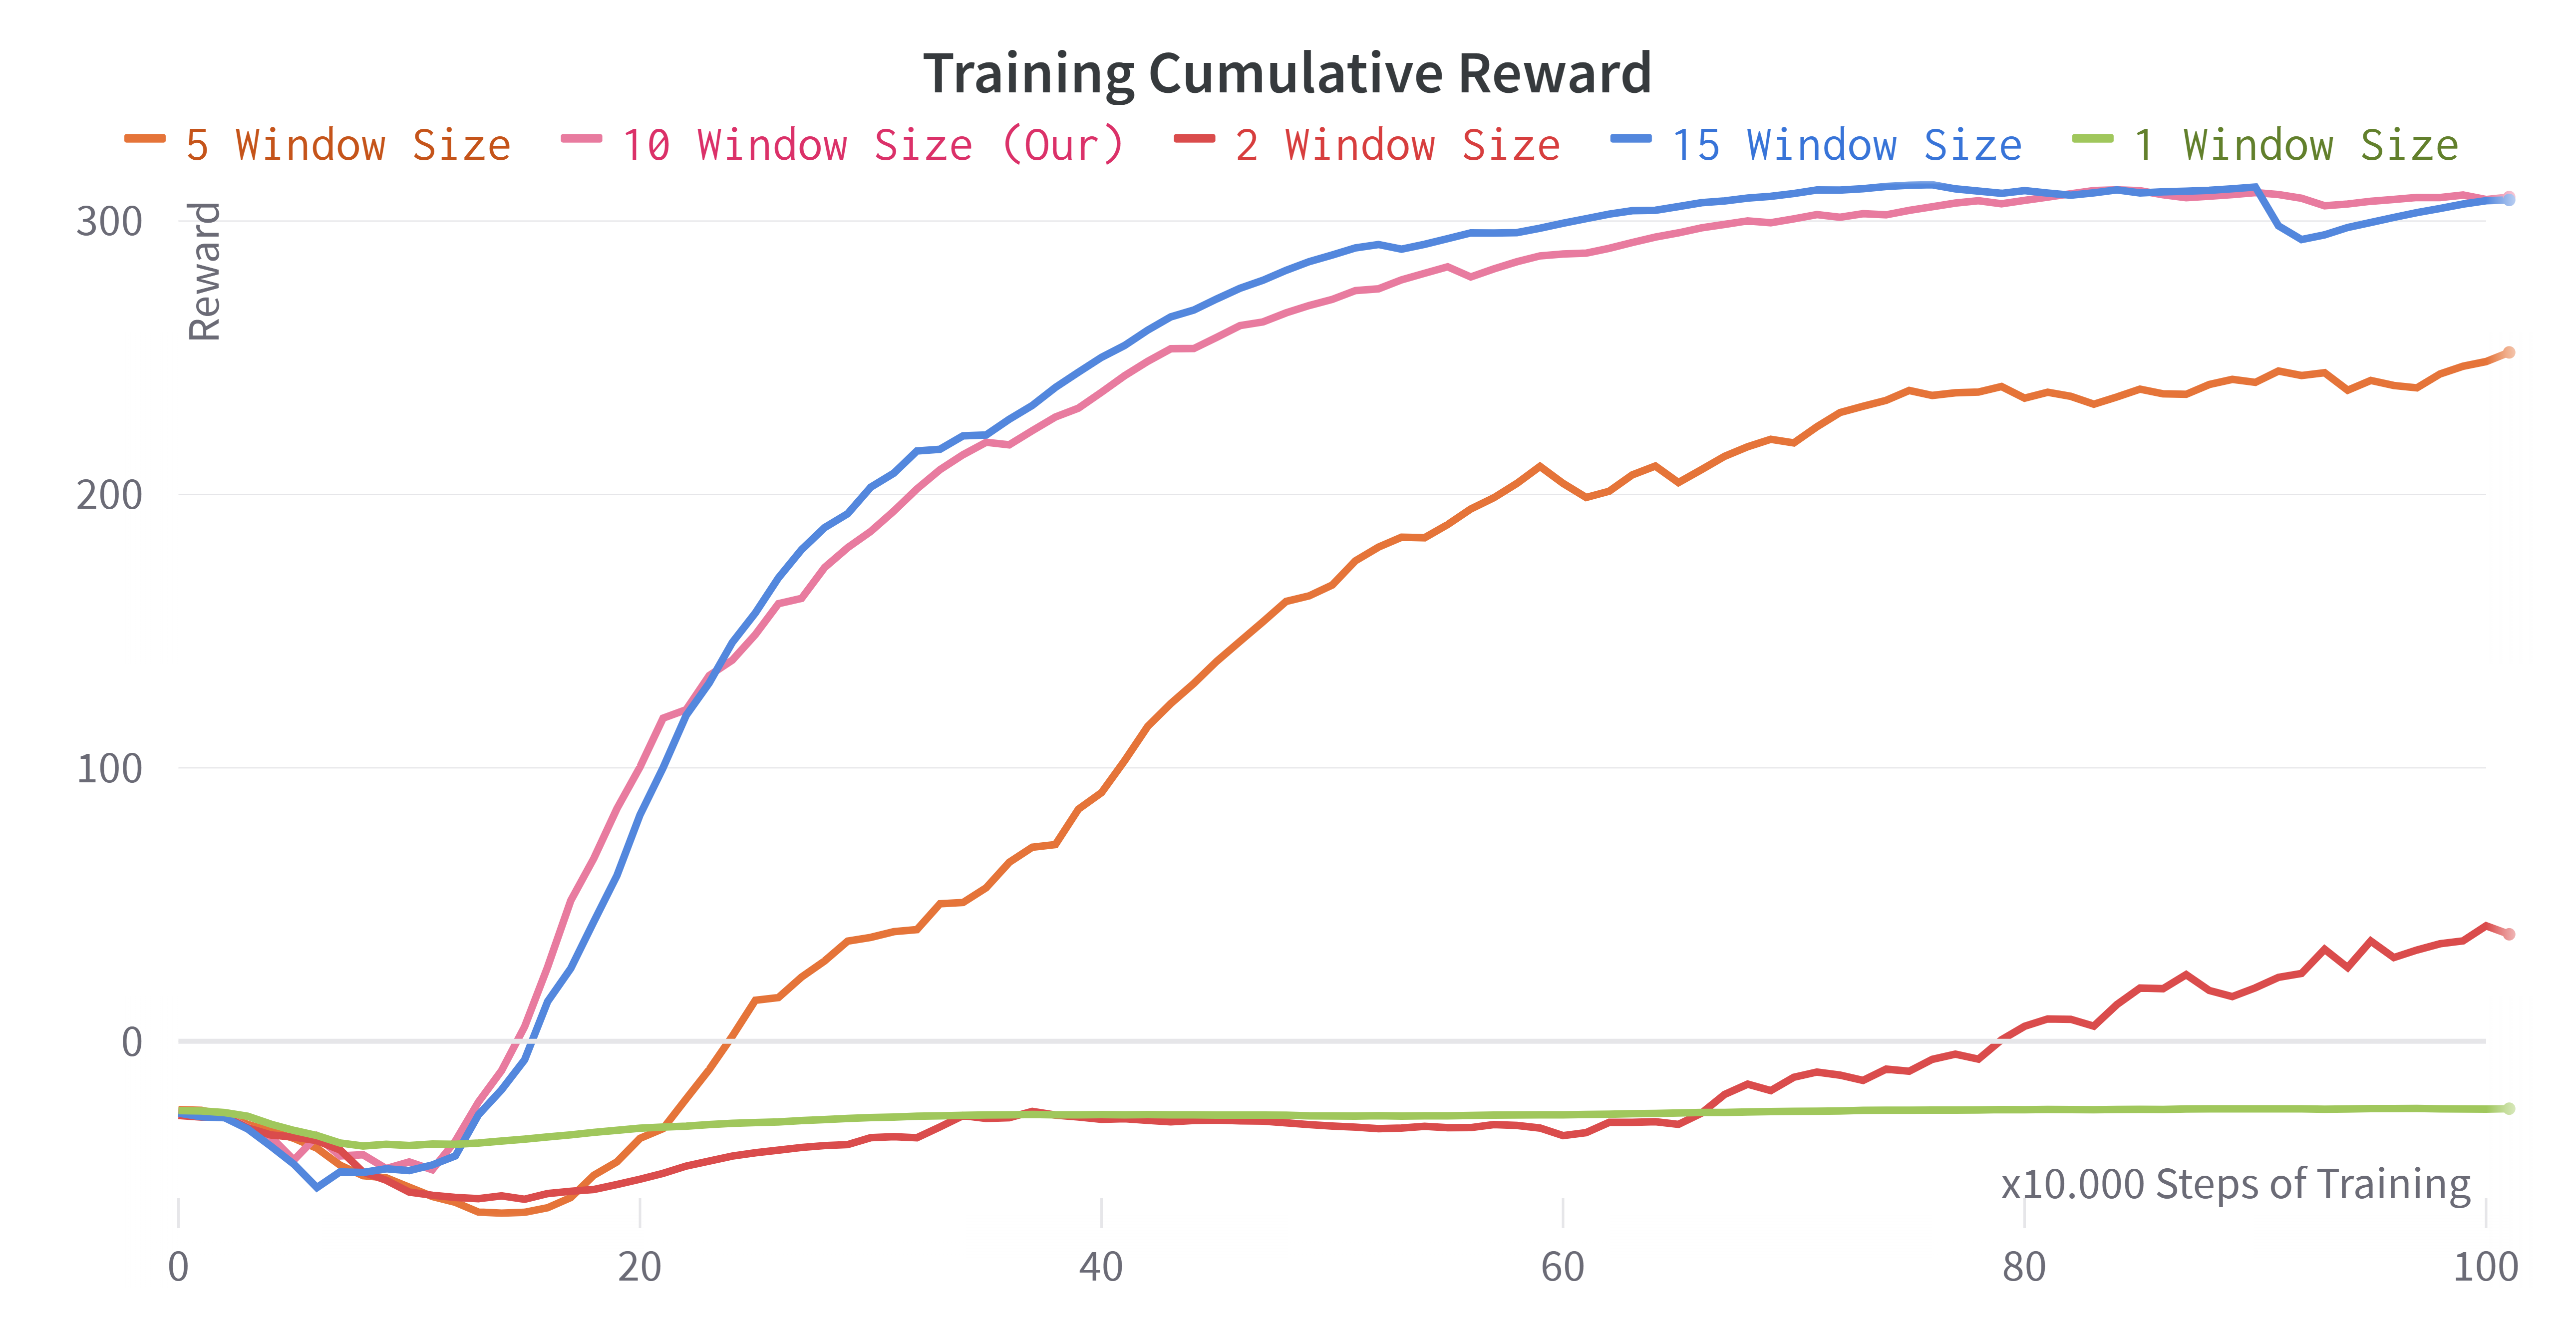}
    \caption{Ablation Study with respect to the length of the observation window. The plot reports the cumulative reward of five training models $\{ \mathbf{e}_\mathbf{w}, \mathbf{R},  \mathbf{u}\}$ characterized by different length of the observation buffer, and taken within the set \{1, 2, 5, 10, 15\}.}
    \label{fig:enter-label}
\end{figure}

\clearpage

\subsection{Velocity Analysis}

\input{tables/velocity_failure}

\subsection{Simulation Experiments}

\begin{table*}[h]

\centering
\caption{Simulation results: positional tracking error in centimeters across different scenarios.}
\resizebox{\textwidth}{!}{
\label{tab:simresults}
\begin{tabular}{|c|c|c|c|c|c|c|c|c|c|c|c|c|c|c|c|c|}
% \cline{2-19}
\hline
% \multirow{3}{*}{\backslashbox{Method}{Scenario}}
% {\backslashbox{Sequence}{Metric}} & $SR$ & $S\text{-}DOD$ & $CE$ & $SR$ & $S\text{-}DOD$ & $CE$ \\
% {\backslashbox{Delay ($\delta$)}{Mass coeff. ($\alpha$)}} & 0.6 & 0.7 & 0.8 & 0.9 & 1.0 & 1.1 & 1.2 & 1.3 & 1.4 &\\
\multirow{3}{*}{\shortstack{Observation\\Space\\Configuration}} & \multicolumn{16}{c|}{Experimental Scenarios and Metrics}\\
\cline{2-17}
& \multicolumn{4}{c|}{Hovering} & \multicolumn{4}{c|}{Planar Ellipse} & \multicolumn{4}{c|}{Planar Eight-Shape} & \multicolumn{4}{c|}{3D Eight-Shape}\\
\cline{2-17}
& $P_{x}$ & $P_{y}$ & $P_{z}$ & $P_{c}$ & $P_{x}$ & $P_{y}$ & $P_{z}$  & $P_{c}$ & $P_{x}$ & $P_{y}$ & $P_{z}$  & $P_{c}$ & $P_{x}$ & $P_{y}$ & $P_{z}$ & $P_{c}$ \\
\hline
$\{ \mathbf{e}_\mathbf{w}, \mathbf{R}, \mathbf{\omega},  \mathbf{u}\}$ & $  \textbf{0.2}$ & $  0.3$ & $  1.3 $ & $ \cellcolor{red!30} 0.6$ & $  4.9$ & $  5.4 $ & $ 1.0 $ & $ \cellcolor{red!30} 3.8$ & $ 2.2$ & $  2.8 $ & $  1.3 $ & $ \cellcolor{red!30} 2.1$ & $  2.5$ & $  2.9 $ & $  1.3 $ & $ \cellcolor{red!30} 2.2$ \\
\hline
$\{ \mathbf{e}_\mathbf{w}, \mathbf{R},  \mathbf{u}\}$ & $  0.3 $ & $  \textbf{0.2} $ & $  0.5$ & $ \cellcolor{green!30} \textbf{0.4}$ & $  1.0 $ & $  2.6 $ & $  1.1$ & $ \cellcolor{yellow!30} 1.5$ & $  1.3 $ & $  1.0 $ & $ 0.9 $ & $ \cellcolor{yellow!30} 1.1$ & $  \textbf{1.1}$ & $ 1.0 $ & $  1.0$ & $ \cellcolor{green!30} \textbf{1.0}$ \\
\hline
$\{ \mathbf{e}_\mathbf{b}, \mathbf{R}, \mathbf{\omega},  \mathbf{u}\}$ & $  0.5 $ & $  0.3 $ & $  0.7 $ & $ \cellcolor{red!30} 0.5$ & $  2.7 $ & $  \textbf{1.9} $ & $  3.3 $ & $ \cellcolor{red!30} 2.6$ & $  2.6 $ & $  1.1 $ & $  1.5 $ & $ \cellcolor{red!30} 1.7$ & $  2.9 $ & $  1.2$ & $  1.8 $ & $ \cellcolor{red!30} 2.0$ \\
\hline
$\{ \mathbf{e}_\mathbf{b}, \mathbf{R},  \mathbf{u}\}$ & $  0.3 $ & $ 0.6 $ & $  \textbf{0.4} $ & $ \cellcolor{yellow!30} 0.5$ & $  1.0 $ & $  2.0 $ & $ 1.3$ & $ \cellcolor{yellow!30} 1.5$ & $  \textbf{1.0} $ & $1.1$ & $  0.8 $ & $ \cellcolor{green!30} 1.0$ & $  \textbf{1.1} $ & $  1.2 $ & $ 1.4 $ & $ \cellcolor{yellow!30} 1.2$ \\
\hline
$\{ \mathbf{e}_\mathbf{b}, \mathbf{\omega},  \mathbf{u}\}$ & $  0.3 $ & $  0.3 $ & $  0.5 $ & $ \cellcolor{green!30} \textbf{0.4}$ & $  1.1 $ & $  2.0 $& $  \textbf{0.6} $& $ \cellcolor{green!30} \textbf{1.2}$& $  1.3 $& $  \textbf{0.8} $& $  \textbf{0.6} $& $ \cellcolor{green!30} \textbf{0.9}$& $  1.3 $& $  \textbf{0.8} $& $  \textbf{0.9} $& $ \cellcolor{green!30} \textbf{1.0}$\\
\hline
$\{ \mathbf{e}_\mathbf{b},  \mathbf{u}\}$ & $ \textbf{0.2}$ & $  0.5$ & $  0.9$ & $ \cellcolor{yellow!30} 0.5$ & $  \textbf{0.9} $ & $  \textbf{1.9} $& $  1.2 $& $ \cellcolor{green!30} 1.3$& $  1.3 $& $  \textbf{0.8} $& $  1.0 $& $ \cellcolor{green!30} 1.0$& $  1.3 $& $  0.9 $& $  1.5 $& $ \cellcolor{yellow!30} 1.2$\\
\hline
\end{tabular}}
\vspace{-1.0em}
\end{table*}

\begin{table*}[h]

\centering
\caption{Simulation results: positional tracking error in centimeters of the experiments conducted at increased speed.}
\resizebox{\textwidth}{!}{
\label{tab:simvelresults}
\begin{tabular}{|c|c|c|c|c|c|c|c|c|c|c|c|c|c|c|c|c|}
% \cline{2-19}
\hline
% \multirow{3}{*}{\backslashbox{Method}{Scenario}}
% {\backslashbox{Sequence}{Metric}} & $SR$ & $S\text{-}DOD$ & $CE$ & $SR$ & $S\text{-}DOD$ & $CE$ \\
% {\backslashbox{Delay ($\delta$)}{Mass coeff. ($\alpha$)}} & 0.6 & 0.7 & 0.8 & 0.9 & 1.0 & 1.1 & 1.2 & 1.3 & 1.4 &\\
\multirow{3}{*}{\shortstack{Observation\\Space\\Configuration}} & \multicolumn{12}{c|}{Experimental Scenarios and Metrics}\\
\cline{2-13} & \multicolumn{4}{c|}{Planar Ellipse} & \multicolumn{4}{c|}{Planar Eight-Shape} & \multicolumn{4}{c|}{3D Eight-Shape}\\
\cline{2-13}
& $P_{x}$ & $P_{y}$ & $P_{z}$ & $P_{c}$ & $P_{x}$ & $P_{y}$ & $P_{z}$  & $P_{c}$ & $P_{x}$ & $P_{y}$ & $P_{z}$  & $P_{c}$ \\
\hline
$\{ \mathbf{e}_\mathbf{w}, \mathbf{R}, \mathbf{\omega},  \mathbf{u}\}$ & $  17.6$ & $  11.1$& $  4.2 $& $ \cellcolor{red!30} 11.0$& $  8.5 $& $  7.5 $& $  2.3 $& $ \cellcolor{red!30} 6.1$& $  10.1 $& $ 7.4$& $  5.7$& $ \cellcolor{red!30} 7.7$ \\
\hline
$\{ \mathbf{e}_\mathbf{w}, \mathbf{R},  \mathbf{u}\}$ & $  \textbf{2.7} $ & $  11.4 $& $  2.3 $& $ \cellcolor{green!30} 5.5$& $ \textbf{3.3}$& $  2.6 $& $  1.5 $& $ \cellcolor{green!30} 2.5$& $  \textbf{2.8} $& $  2.8 $& $  \textbf{4.0}$& $ \cellcolor{green!30} \textbf{3.2}$ \\
\hline
$\{ \mathbf{e}_\mathbf{b}, \mathbf{R}, \mathbf{\omega},  \mathbf{u}\}$ & $  5.3 $ & $  15.8 $& $  9.4 $& $ \cellcolor{red!30} 10.2$& $  5.4 $& $  2.4 $& $  3.2$& $ \cellcolor{red!30} 3.7$& $  6.0$& $  2.7 $& $  6.2$& $ \cellcolor{red!30} 4.9$ \\
\hline
$\{ \mathbf{e}_\mathbf{b}, \mathbf{R},  \mathbf{u}\}$ & $  3.9 $ & $  10.6 $& $  4.3 $& $ \cellcolor{yellow!30} 6.3$& $  4.5 $& $  \textbf{1.9}$& $  2.3$& $ \cellcolor{yellow!30} 2.9$& $  5.2$& $  \textbf{1.9} $& $  5.5 $& $ \cellcolor{yellow!30} 4.2$ \\
\hline
$\{ \mathbf{e}_\mathbf{b}, \mathbf{\omega},  \mathbf{u}\}$ & $  7.2 $ & $  9.2 $& $  2.2 $& $ \cellcolor{yellow!30} 6.2$& $  4.2 $& $  2.1 $& $  \textbf{0.8} $& $ \cellcolor{green!30} \textbf{2.4}$& $  4.1 $& $  2.7 $& $  4.3 $& $ \cellcolor{green!30} 3.7$ \\
\hline
$\{ \mathbf{e}_\mathbf{b},  \mathbf{u}\}$  & $  5.2 $ & $  \textbf{8.0} $& $  \textbf{1.8} $& $ \cellcolor{green!30} \textbf{5.0}$& $  5.9 $& $  2.4 $& $  2.3 $& $ \cellcolor{yellow!30} 3.6$& $  5.9 $& $  2.8 $& $  5.6 $& $ \cellcolor{yellow!30} 4.8$ \\
\hline
\end{tabular}}
\vspace{-1.0em}
\end{table*}

\clearpage
\subsection{Effort Analysis}

\begin{table*}[h]

\centering
\caption{Mean of the accumulated angular velocities in rad/s across different scenarios.}
\resizebox{\textwidth}{!}{
\label{tab:simresults}
\begin{tabular}{|c|c|c|c|c|c|c|c|c|c|c|c|c|c|c|c|c|}
% \cline{2-19}
\hline
% \multirow{3}{*}{\backslashbox{Method}{Scenario}}
% {\backslashbox{Sequence}{Metric}} & $SR$ & $S\text{-}DOD$ & $CE$ & $SR$ & $S\text{-}DOD$ & $CE$ \\
% {\backslashbox{Delay ($\delta$)}{Mass coeff. ($\alpha$)}} & 0.6 & 0.7 & 0.8 & 0.9 & 1.0 & 1.1 & 1.2 & 1.3 & 1.4 &\\
\multirow{3}{*}{\shortstack{Observation\\Space\\Configuration}} & \multicolumn{16}{c|}{Experimental Scenarios and Metrics}\\
\cline{2-17}
& \multicolumn{4}{c|}{Hovering} & \multicolumn{4}{c|}{Planar Ellipse} & \multicolumn{4}{c|}{Planar Eight-Shape} & \multicolumn{4}{c|}{3D Eight-Shape}\\
\cline{2-17}
& $A_{\omega x}$ & $A_{\omega y}$ & $A_{\omega z}$ & $A_{c}$ & $A_{\omega x}$ & $A_{\omega y}$ & $A_{\omega z}$ & $A_{c}$ & $A_{\omega x}$ & $A_{\omega y}$ & $A_{\omega z}$ & $A_{c}$ & $A_{\omega x}$ & $A_{\omega y}$ & $A_{\omega z}$ & $A_{c}$ \\
\hline
$\{ \mathbf{e}_\mathbf{w}, \mathbf{R}, \mathbf{\omega},  \mathbf{u}\}$ & $  0.07$ & $  0.04$ & $  0.04 $ & $ \cellcolor{green!30} 0.05$ & $  0.10$ & $  0.10 $ & $ 0.09 $ & $ \cellcolor{green!30} 0.10$ & $ 0.08$ & $  0.07 $ & $  0.07 $ & $ \cellcolor{green!30} 0.07$ & $  0.09$ & $  0.07 $ & $  0.06 $ & $ \cellcolor{green!30} 0.07$ \\
\hline
$\{ \mathbf{e}_\mathbf{w}, \mathbf{R},  \mathbf{u}\}$ & $  0.06 $ & $  0.08 $ & $  0.04$ & $ \cellcolor{yellow!30} 0.06$ & $  0.13 $ & $  0.10 $ & $  0.09$ & $ \cellcolor{yellow!30} 0.11$ & $  0.08 $ & $  0.10 $ & $ 0.05 $ & $ \cellcolor{yellow!30} 0.08$ & $  0.08$ & $ 0.09 $ & $  0.05$ & $ \cellcolor{green!30} 0.07$ \\
\hline
$\{ \mathbf{e}_\mathbf{b}, \mathbf{R}, \mathbf{\omega},  \mathbf{u}\}$ & $  0.03 $ & $  0.04 $ & $  0.06 $ & $ \cellcolor{green!30} 0.04$ & $  0.12 $ & $  0.12 $ & $  0.25 $ & $ \cellcolor{red!30} 0.17$ & $  0.06 $ & $  0.07 $ & $  0.15 $ & $ \cellcolor{red!30} 0.09$ & $  0.07 $ & $  0.09$ & $  0.17 $ & $ \cellcolor{red!30} 0.11$ \\
\hline
$\{ \mathbf{e}_\mathbf{b}, \mathbf{R},  \mathbf{u}\}$ & $  0.06 $ & $ 0.07 $ & $  0.07 $ & $ \cellcolor{yellow!30} 0.06$ & $  0.13 $ & $  0.11 $ & $ 0.21$ & $ \cellcolor{red!30} 0.15$ & $  0.08 $ & $0.09$ & $  0.12 $ & $ \cellcolor{red!30} 0.10$ & $  0.08 $ & $  0.10 $ & $ 0.14 $ & $ \cellcolor{red!30} 0.10$ \\
\hline
$\{ \mathbf{e}_\mathbf{b}, \mathbf{\omega},  \mathbf{u}\}$ & $  0.06 $ & $  0.05 $ & $  0.02 $ & $ \cellcolor{green!30} 0.05$ & $  0.14 $ & $  0.11 $& $  0.07 $& $ \cellcolor{green!30} 0.10$& $  0.08 $& $  0.08 $& $  0.04 $& $ \cellcolor{green!30} 0.07$& $  0.09 $& $  0.09 $& $  0.05 $& $ \cellcolor{yellow!30} 0.08$\\
\hline
$\{ \mathbf{e}_\mathbf{b},  \mathbf{u}\}$ & $ 0.10$ & $  0.06$ & $  0.05$ & $ \cellcolor{red!30} 0.07$ & $  0.13 $ & $  0.09 $& $  0.08 $& $ \cellcolor{green!30} 0.10$& $  0.11 $& $  0.08 $& $  0.06 $& $ \cellcolor{yellow!30} 0.08$& $  0.11 $& $  0.08 $& $  0.06 $& $ \cellcolor{yellow!30} 0.08$\\
\hline
\end{tabular}}
\vspace{-1.0em}
\end{table*}

\clearpage
\subsection{Updated Tables}
\begin{table*}[h]

\centering
\caption{Experimental results: positional tracking error in centimeters across different scenarios.}
\resizebox{\textwidth}{!}{
\label{tab:results}
\begin{tabular}{|c|c|c|c|c|c|c|c|c|c|c|c|c|c|c|c|c|}
% \cline{2-19}
\hline
% \multirow{3}{*}{\backslashbox{Method}{Scenario}}
% {\backslashbox{Sequence}{Metric}} & $SR$ & $S\text{-}DOD$ & $CE$ & $SR$ & $S\text{-}DOD$ & $CE$ \\
% {\backslashbox{Delay ($\delta$)}{Mass coeff. ($\alpha$)}} & 0.6 & 0.7 & 0.8 & 0.9 & 1.0 & 1.1 & 1.2 & 1.3 & 1.4 &\\
\multirow{3}{*}{\shortstack{Observation\\Space\\Configuration}} & \multicolumn{16}{c|}{Experimental Scenarios and Metrics}\\
\cline{2-17}
& \multicolumn{4}{c|}{Hovering} & \multicolumn{4}{c|}{Planar Ellipse} & \multicolumn{4}{c|}{Planar Eight-Shape} & \multicolumn{4}{c|}{3D Eight-Shape}\\
\cline{2-17}
& $P_{x}$ & $P_{y}$ & $P_{z}$ & $P_{c}$ & $P_{x}$ & $P_{y}$ & $P_{z}$  & $P_{c}$ & $P_{x}$ & $P_{y}$ & $P_{z}$  & $P_{c}$ & $P_{x}$ & $P_{y}$ & $P_{z}$ & $P_{c}$ \\
\hline
$\{ \mathbf{e}_\mathbf{w}, \mathbf{R}, \mathbf{\omega},  \mathbf{u}\}$ & $  5.0$ & $  6.9$ & $  \textbf{2.1} $ & $ \cellcolor{red!30} 4.6$ & $  7.9$ & $  6.6 $ & $ \textbf{2.7} $ & $ \cellcolor{red!30} 5.7$ & $ 9.8$ & $  7.1 $ & $  3.4 $ & $ \cellcolor{red!30} 6.8$ & $  9.6$ & $  8.5 $ & $  6.0 $ & $ \cellcolor{red!30} 8.1$ \\
\hline
$\{ \mathbf{e}_\mathbf{w}, \mathbf{R},  \mathbf{u}\}$ & $  2.6 $ & $  \textbf{2.1} $ & $  3.3$ & $ \cellcolor{green!30} \textbf{2.7}$ & $  \textbf{2.3} $ & $  3.4 $ & $  3.2$ & $ \cellcolor{green!30} \textbf{3.0}$ & $  \textbf{2.7} $ & $  \textbf{2.8} $ & $ 4.1 $ & $ \cellcolor{green!30} \textbf{3.1}$ & $  \textbf{2.5}$ & $ 2.9 $ & $  6.2$ & $ \cellcolor{green!30} \textbf{3.9}$ \\
\hline
$\{ \mathbf{e}_\mathbf{b}, \mathbf{R}, \mathbf{\omega},  \mathbf{u}\}$ & $  4.7 $ & $  3.0 $ & $  3.2 $ & $ \cellcolor{red!30} 3.7$ & $  6.7 $ & $  4.2 $ & $  4.4 $ & $ \cellcolor{red!30} 5.1$ & $  9.5 $ & $  3.1 $ & $  \textbf{3.1} $ & $ \cellcolor{red!30} 5.2$ & $  8.0 $ & $  2.9$ & $  6.6 $ & $ \cellcolor{red!30} 5.8$ \\
\hline
$\{ \mathbf{e}_\mathbf{b}, \mathbf{R},  \mathbf{u}\}$ & $  2.5 $ & $ 2.7 $ & $  3.1 $ & $ \cellcolor{green!30} \textbf{2.7}$ & $  4.0 $ & $  \textbf{3.3} $ & $ 3.6$ & $ \cellcolor{green!30} 3.6$ & $  4.1 $ & $3.0 $ & $  3.6 $ & $ \cellcolor{green!30} 3.5$ & $  3.1 $ & $  \textbf{2.6} $ & $ \textbf{5.8} $ & $ \cellcolor{green!30} \textbf{3.9}$ \\
\hline
$\{ \mathbf{e}_\mathbf{b}, \mathbf{\omega},  \mathbf{u}\}$ & $  \textbf{2.1} $ & $  3.2 $ & $  2.7 $ & $ \cellcolor{green!30} \textbf{2.7}$ & $  3.7 $ & $  5.0 $ & $  3.2$ & $ \cellcolor{yellow!30} 4.0$ & $  3.5$ & $  4.2 $  & $ 3.3 $ & $ \cellcolor{yellow!30} 3.6$ & $  4.2 $ & $  4.5 $ & $  \textbf{5.8} $ & $ \cellcolor{yellow!30} 4.8$\\
\hline
$\{ \mathbf{e}_\mathbf{b},  \mathbf{u}\}$ & $ 2.2$ & $  3.7$ & $  3.1$ & $ \cellcolor{yellow!30} 3.0$ & $  3.2$ & $  4.7$ & $  3.0$ & $ \cellcolor{green!30} 3.6$ & $  3.3$ & $  4.2 $  & $  3.9 $ & $ \cellcolor{yellow!30} 3.8$ & $  3.5$ & $  4.3$ & $ 6.7$ & $ \cellcolor{yellow!30} 4.8$\\
\hline
\hline
PID Controller & $ 1.6$ & $  1.5$ & $  1.4$ & $ \cellcolor{green!30} 1.5$ & $  2.4$ & $  5.5$ & $  1.6$ & $ \cellcolor{green!30} 3.2$ & $  2.8$ & $  2.7 $  & $  1.5 $ & $ \cellcolor{green!30} 2.3$ & $  3.4$ & $  2.6$ & $ 8.7$ & $ \cellcolor{yellow!30} 4.9$\\
\hline
\end{tabular}}
\vspace{-1.0em}
\end{table*}
\begin{table*}[h]

\centering
\caption{Positional tracking error in centimeters of the experiments conducted at increased speed.}
\resizebox{0.7\textwidth}{!}{
\label{tab:velresults}
\begin{tabular}{|c|c|c|c|c|c|c|c|c|c|c|c|c|c|c|c|c|}
% \cline{2-19}
\hline
% \multirow{3}{*}{\backslashbox{Method}{Scenario}}
% {\backslashbox{Sequence}{Metric}} & $SR$ & $S\text{-}DOD$ & $CE$ & $SR$ & $S\text{-}DOD$ & $CE$ \\
% {\backslashbox{Delay ($\delta$)}{Mass coeff. ($\alpha$)}} & 0.6 & 0.7 & 0.8 & 0.9 & 1.0 & 1.1 & 1.2 & 1.3 & 1.4 &\\
\multirow{3}{*}{\shortstack{Observation\\Space\\Configuration}} & \multicolumn{12}{c|}{Experimental Scenarios and Metrics}\\
\cline{2-13} & \multicolumn{4}{c|}{Planar Ellipse} & \multicolumn{4}{c|}{Planar Eight-Shape} & \multicolumn{4}{c|}{3D Eight-Shape}\\
\cline{2-13}
& $P_{x}$ & $P_{y}$ & $P_{z}$ & $P_{c}$ & $P_{x}$ & $P_{y}$ & $P_{z}$  & $P_{c}$ & $P_{x}$ & $P_{y}$ & $P_{z}$  & $P_{c}$ \\
\hline
$\{ \mathbf{e}_\mathbf{w}, \mathbf{R}, \mathbf{\omega},  \mathbf{u}\}$ & $  18.3$ & $  10.4$& $  3.5 $& $ \cellcolor{red!30} 10.7$& $  13.8 $& $  10.4 $& $  5.0 $& $ \cellcolor{red!30} 9.7$& $  15.0 $& $ 10.3$& $  6.9$& $ \cellcolor{red!30} 10.7$ \\
\hline
$\{ \mathbf{e}_\mathbf{w}, \mathbf{R},  \mathbf{u}\}$ & $  \textbf{3.6} $ & $  10.9 $& $  3.8 $& $ \cellcolor{green!30} \textbf{6.1}$& $ \textbf{4.0}$& $  \textbf{3.6} $& $  4.3 $& $ \cellcolor{green!30} \textbf{4.0}$& $  \textbf{3.8} $& $  \textbf{3.9} $& $  5.7$& $ \cellcolor{green!30} \textbf{4.5}$ \\
\hline
$\{ \mathbf{e}_\mathbf{b}, \mathbf{R}, \mathbf{\omega},  \mathbf{u}\}$ & $  7.2 $ & $  15.6 $& $  9.2 $& $ \cellcolor{red!30} 10.7$& $  9.9 $& $  4.4 $& $  4.5$& $ \cellcolor{red!30} 6.3$& $  10.3$& $  4.7 $& $  7.5$& $ \cellcolor{red!30} 7.5$ \\
\hline
$\{ \mathbf{e}_\mathbf{b}, \mathbf{R},  \mathbf{u}\}$ & $  7.7 $ & $  11.8 $& $  7.0 $& $ \cellcolor{yellow!30} 8.8$& $  7.0 $& $  4.9$& $  4.2$& $ \cellcolor{yellow!30} 5.4$& $  8.5$& $  6.1 $& $  6.8 $& $ \cellcolor{yellow!30} 7.1$ \\
\hline
$\{ \mathbf{e}_\mathbf{b}, \mathbf{\omega},  \mathbf{u}\}$ & $  9.1 $ & $  \textbf{9.6} $& $  4.0 $& $ \cellcolor{yellow!30} 7.6$& $  4.4 $& $  5.7 $& $  \textbf{3.1} $& $ \cellcolor{green!30} 4.3$& $  5.5 $& $  6.4 $& $  5.9 $& $ \cellcolor{yellow!30} 5.9$ \\
\hline
$\{ \mathbf{e}_\mathbf{b},  \mathbf{u}\}$  & $  7.3 $ & $  10.1 $& $  \textbf{2.9} $& $ \cellcolor{green!30} 6.8$& $  7.0 $& $  7.2 $& $  3.3 $& $ \cellcolor{yellow!30} 5.9$& $  5.0 $& $  6.9 $& $  \textbf{4.7} $& $ \cellcolor{green!30} 5.5$ \\
\hline
\hline
PID Controller  & $  7.8 $ & $  15.6 $& $  2.2 $& $ \cellcolor{yellow!30} 8.5$& $  7.9 $& $  5.8 $& $  1.5 $& $ \cellcolor{yellow!30} 5.1$& $  8.2 $& $  5.8 $& $  16.8 $& $ \cellcolor{red!30} 10.3$ \\
\hline
\end{tabular}}
\vspace{-1.0em}
\end{table*}

\clearpage
\subsection{Convergence comparison}

\begin{figure}[h]
    \centering
    \includegraphics[width=\textwidth]{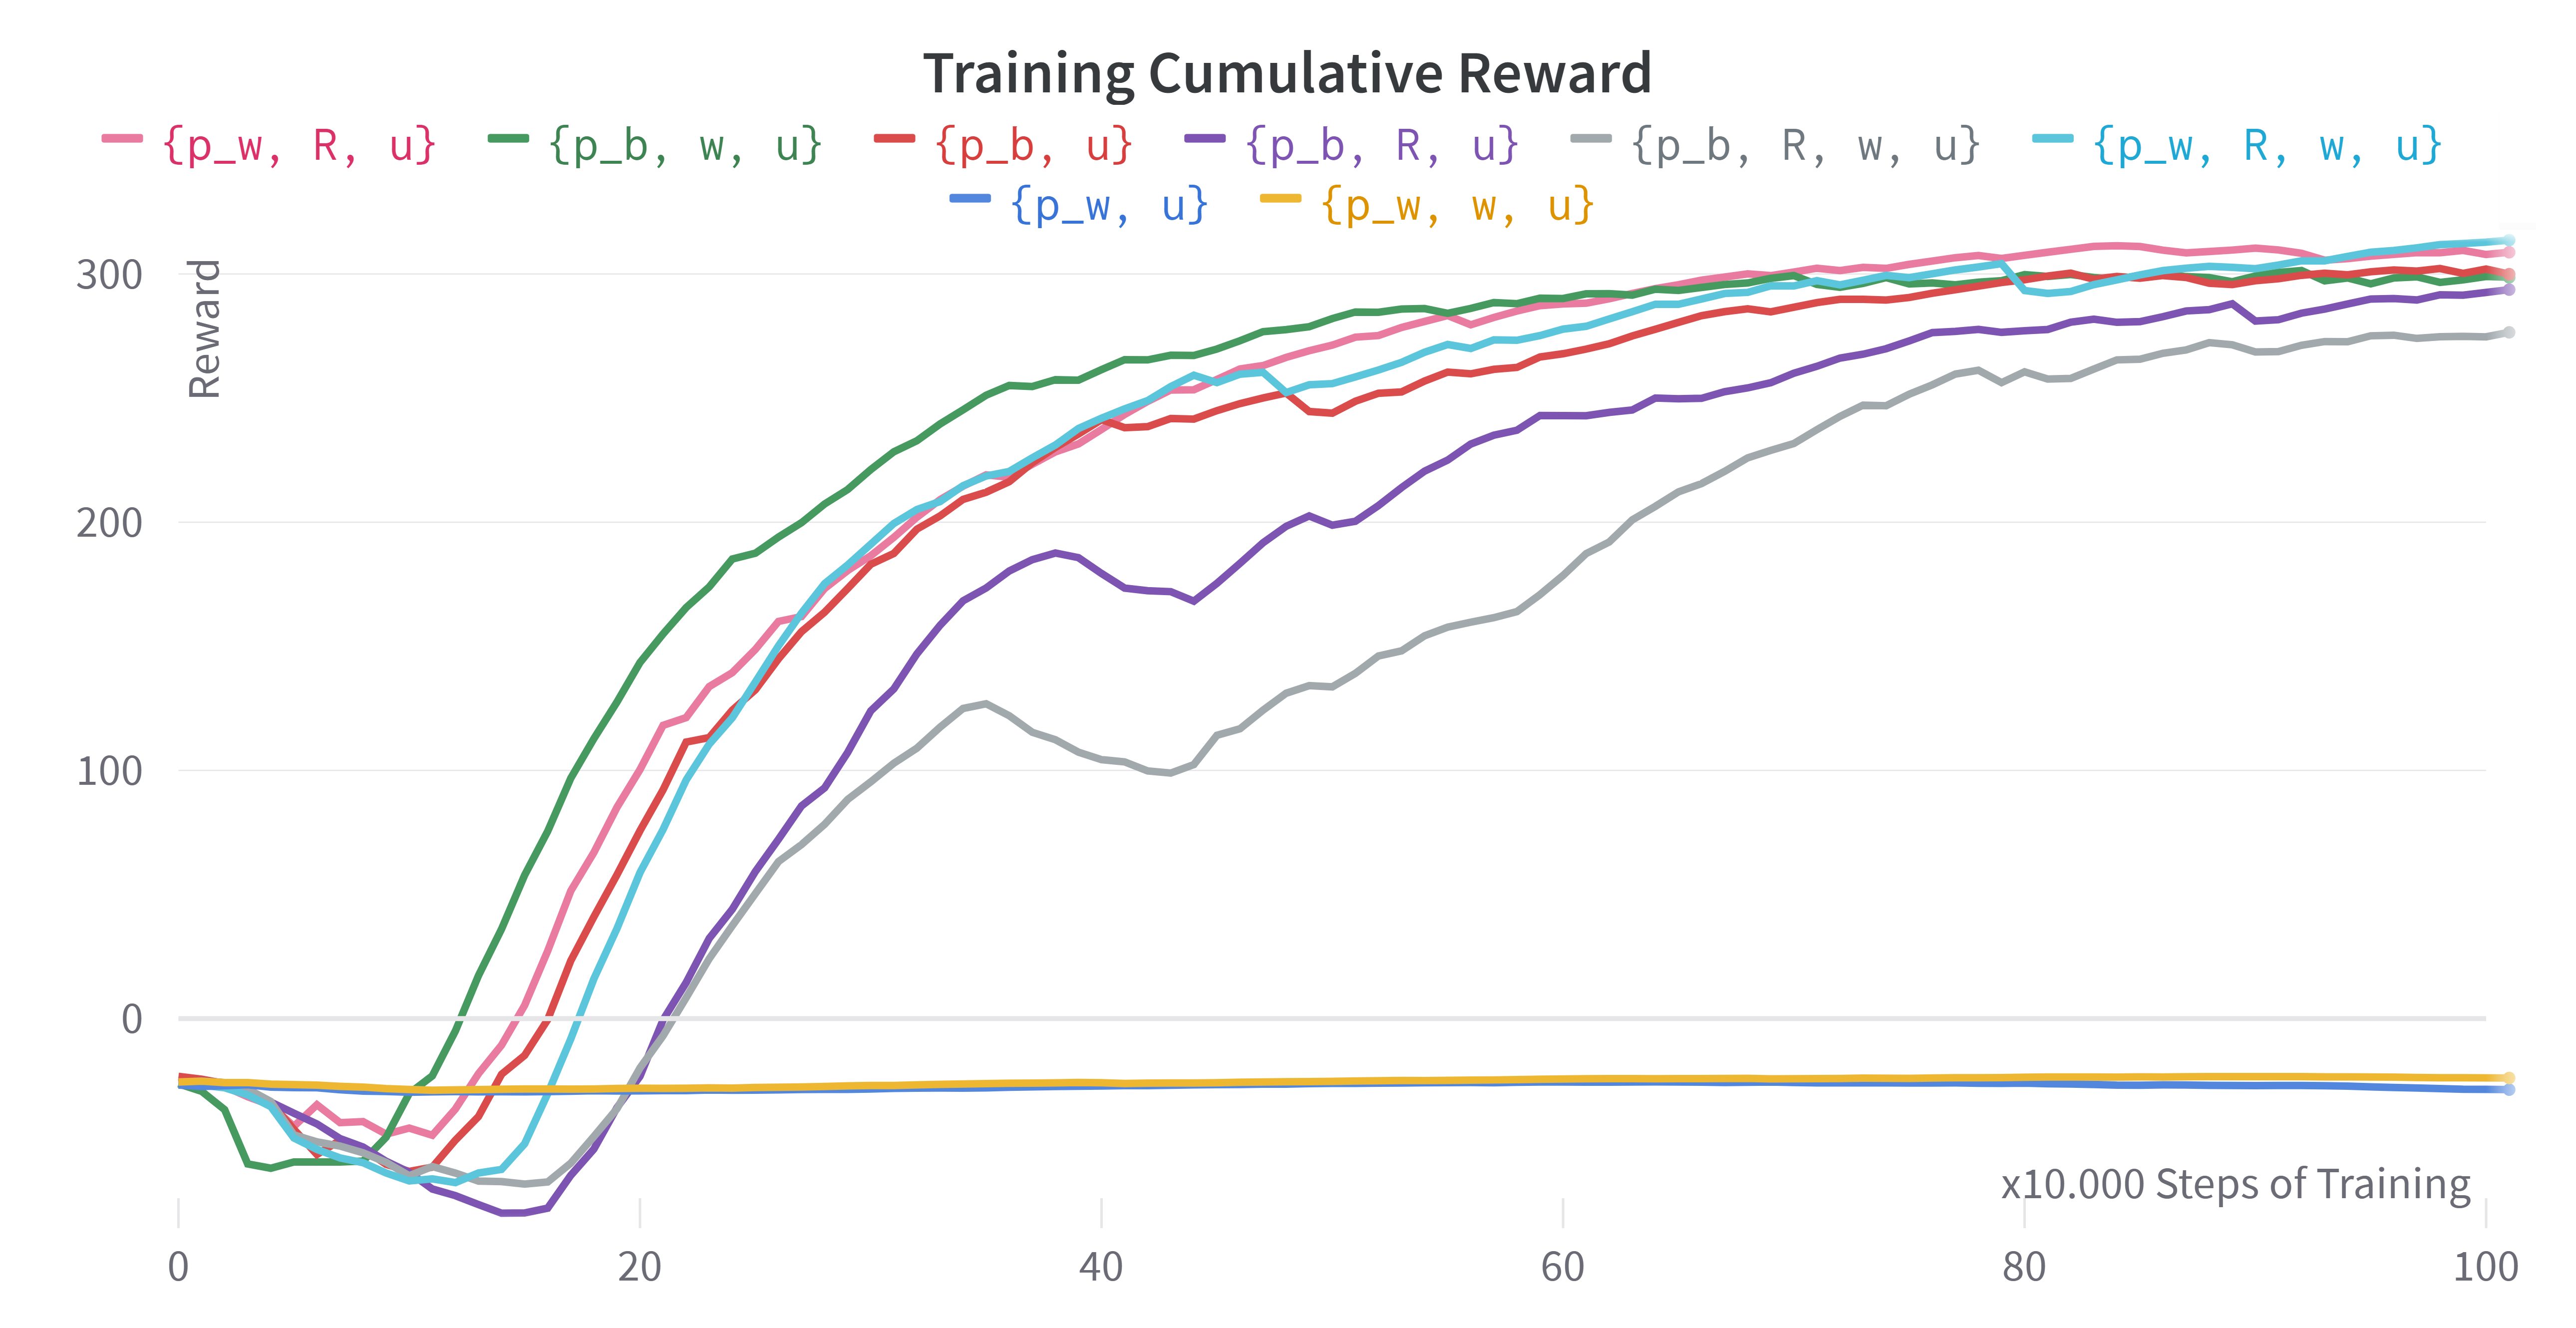}
    \caption{The plot reports the cumulative reward of the models considered in the benchmark study.}
    \label{fig:enter-label}
\end{figure}
